# Supplementary material for: Sub-wavelength spin excitations in ultracold gases created by stimulated Raman transitions
Source: arXiv:2004.05044 ancillary file (2020-04-10)
Supplement: Supplementary file 1 [file supplementary_material.pdf]

# Sub-wavelength spin excitations in ultracold gases created by stimulated Raman transitions

## Supplementary Material

*Yigal Ilin, Shai Tsesses, Guy Bartal and Yoav Sagi*

### S1: Model outline and derivation

The combined optical field has the form:

$$\begin{aligned}\vec{E}(\vec{r},t)&=\vec{E}_1(\vec{r},t)+\vec{E}_2(\vec{r},t)=\\&=\vec{\varepsilon}_1(x,y)e^{-|k_{1,z}|z}e^{j\omega_1 t}+\vec{\varepsilon}_2(x,y)e^{-|k_{2,z}|z}e^{j\omega_2 t}\end{aligned}\qquad(1)$$

Above field can be decomposed in terms of rotating and counter rotating components: $\vec{E}_\alpha=\vec{E}_\alpha^{(+)}+\vec{E}_\alpha^{(-)}$ where $\vec{E}_\alpha^{(+)}\propto e^{-j\omega_\alpha t}$, $\vec{E}_\alpha^{(-)}\propto e^{+j\omega_\alpha t}$ and $\alpha=1,2$. We also define phase vector for the field $\alpha$ as $\vec{E}_\alpha(\vec{r})=\mathrm{Re}\left\{\tilde{\vec{E}}_\alpha(\vec{r})e^{j\omega_\alpha t}\right\}$.

This leads to the following:

$$\begin{aligned}\vec{E}^{(+)}&=\frac{1}{2}\tilde{\vec{E}}_1(\vec{r})e^{-j\omega_1 t}+\frac{1}{2}\tilde{\vec{E}}_2(\vec{r})e^{-j\omega_2 t}\\\vec{E}^{(-)}&=\frac{1}{2}\tilde{\vec{E}}_1(\vec{r})e^{+j\omega_1 t}+\frac{1}{2}\tilde{\vec{E}}_2(\vec{r})e^{+j\omega_2 t}\end{aligned}\qquad(2)$$

### S1.1: Defining Rabi frequencies and dipole matrix elements

Developing atom-field Hamiltonian using rotating wave approximation for the fields above:

$$\begin{aligned}H_{AF}&=-\frac{1}{2}\left(\langle g_1|\vec{d}|e\rangle\sigma_1\cdot\tilde{\vec{E}}_1^*(\vec{r})e^{+j\omega_1 t}+\langle g_2|\vec{d}|e\rangle\sigma_2\cdot\tilde{\vec{E}}_2^*(\vec{r})e^{+j\omega_2 t}\right)-\\&-\frac{1}{2}\left(\langle g_1|\vec{d}|e\rangle\sigma_1^\dagger\cdot\tilde{\vec{E}}_1(\vec{r})e^{-j\omega_1 t}+\langle g_2|\vec{d}|e\rangle\sigma_2^\dagger\cdot\tilde{\vec{E}}_2(\vec{r})e^{-j\omega_2 t}\right)=\\&=-\frac{1}{2}\left(\langle g_1|\vec{d}|e\rangle\sigma_1\cdot\tilde{\vec{E}}_1^*(\vec{r})e^{+j\omega_1 t}+\langle g_1|\vec{d}|e\rangle\sigma_1^\dagger\cdot\tilde{\vec{E}}_1(\vec{r},\vec{k}_1)e^{-j\omega_1 t}\right)-\\&-\frac{1}{2}\left(\langle g_2|\vec{d}|e\rangle\sigma_2\cdot\tilde{\vec{E}}_2^*(\vec{r})e^{+j\omega_2 t}+\langle g_2|\vec{d}|e\rangle\sigma_2^\dagger\cdot\tilde{\vec{E}}_2(\vec{r})e^{-j\omega_2 t}\right)=\\&=-\frac{1}{2}\langle g_1|\vec{d}|e\rangle\sigma_1\cdot\tilde{\vec{E}}_1^*(\vec{r})e^{+j\omega_1 t}-\frac{1}{2}\langle g_2|\vec{d}|e\rangle\sigma_2\cdot\tilde{\vec{E}}_2^*(\vec{r})e^{+j\omega_2 t}+h.c.\end{aligned}\qquad(3)$$

where $\sigma_\alpha=|g_\alpha\rangle\langle e|$ is the transition operator.

Now we define two Rabi frequencies as following:

$$\Omega_1(\vec{r}) = -\frac{1}{\hbar}\langle g_1|\vec{d}|e\rangle \cdot \vec{\tilde{E}}_1^*(\vec{r})$$
$$\Omega_2(\vec{k}_2) = -\frac{1}{\hbar}\langle g_2|\vec{d}|e\rangle \cdot \vec{\tilde{E}}_2^*(\vec{r}) \qquad (4)$$

Introduce the following spherical unit vectors:

$$\hat{u}_{+1} = \frac{\hat{x}+i\hat{y}}{\sqrt{2}},\ \hat{u}_{-1} = \frac{\hat{x}-i\hat{y}}{\sqrt{2}},\ \hat{u}_0 = \hat{z}$$
$$\hat{x} = \frac{\hat{u}_{+1}+\hat{u}_{-1}}{\sqrt{2}},\ \hat{y} = \frac{\hat{u}_{+1}-\hat{u}_{-1}}{i\sqrt{2}},\ \hat{z} = \hat{u}_0 \qquad (5)$$

Expressing $\vec{\tilde{E}}_\alpha$ with (5), yields:

$$\begin{aligned}\vec{\tilde{E}}_\alpha(\vec{r}) &= \tilde{E}_{\alpha,x}(\vec{r})\hat{x} + \tilde{E}_{\alpha,y}(\vec{r})\hat{y} + \tilde{E}_{\alpha,z}(\vec{r})\hat{z} = \\ &= \tilde{E}_{\alpha,x}(\vec{r})\left(\frac{\hat{u}_{+1}+\hat{u}_{-1}}{\sqrt{2}}\right) + \tilde{E}_{\alpha,y}(\vec{r})\left(\frac{\hat{u}_{+1}-\hat{u}_{-1}}{i\sqrt{2}}\right) + \tilde{E}_{\alpha,z}(\vec{r})\hat{u}_0 = \\ &= \frac{1}{\sqrt{2}}\left[\tilde{E}_{\alpha,x}(\vec{r}) - i\tilde{E}_{\alpha,y}(\vec{r})\right]\hat{u}_{+1} + \frac{1}{\sqrt{2}}\left[\tilde{E}_{\alpha,x}(\vec{r}) + i\tilde{E}_{\alpha,y}(\vec{r})\right]\hat{u}_{-1} + \tilde{E}_{\alpha,z}(\vec{r})\hat{u}_0\end{aligned} \qquad (6)$$

Now we write (4) in an explicit way:

$$\begin{aligned}\Omega_\alpha(\vec{r},\vec{k}_1) &= -\frac{1}{\hbar}\langle g_\alpha|\vec{d}|e\rangle \cdot \vec{\tilde{E}}_\alpha^*(\vec{r}) = \\ &= -\frac{1}{\hbar\sqrt{2}}\langle g_\alpha|\vec{d}\cdot\hat{u}_{+1}|e\rangle\left[\tilde{E}_{\alpha,x}^*(\vec{r}) - i\tilde{E}_{\alpha,y}^*(\vec{r})\right] - \\ &- \frac{1}{\hbar\sqrt{2}}\langle g_\alpha|\vec{d}\cdot\hat{u}_{-1}|e\rangle\left[\tilde{E}_{\alpha,x}^*(\vec{r}) + i\tilde{E}_{\alpha,y}^*(\vec{r})\right] - \frac{1}{\hbar}\langle g_\alpha|\vec{d}\cdot\hat{u}_0|e\rangle\tilde{E}_{\alpha,z}^*(\vec{r})\end{aligned} \qquad (7)$$

Using this spherical basis, the expression for the matrix element:

$$\begin{aligned}&\vec{r}\cdot\hat{u}_q = \sqrt{\frac{4\pi}{3}}rY_{1,q}(\theta,\phi) \Rightarrow \\ &\Rightarrow \langle g_\alpha|\vec{d}\cdot\hat{u}_q|e\rangle = -q_e\iiint r^2\sin\theta drd\theta d\phi\left[\psi_{g_\alpha}^*(r,\theta,\phi)\sqrt{\frac{4\pi}{3}}rY_{1,q}(\theta,\phi)\psi_e(r,\theta,\phi)\right]\end{aligned} \qquad (8)$$

## **S1.2: Translating the atom-field Hamiltonian into rotating frames of the fields**

Writing the (3) with Rabi frequencies:

$$H_{AF} = \frac{\hbar}{2}\left[\Omega_1(\vec{r})\sigma_1 e^{+j\omega_1 t} + \Omega_1^*(\vec{r})\sigma_1^\dagger e^{-j\omega_1 t}\right] + \frac{\hbar}{2}\left[\Omega_2(\vec{r})\sigma_2 e^{+j\omega_2 t} + \Omega_2^*(\vec{r})\sigma_2^\dagger e^{-j\omega_2 t}\right] \qquad (9)$$

Write out general state as super-position of internal states:

$$|\psi\rangle = c_1|g_1\rangle + c_2|g_2\rangle + c_e|e\rangle \qquad (10)$$

Transform the above into the rotating frames of the two electric fields:

$$|\psi\rangle = c_1|g_1\rangle + c_2|g_2\rangle + c_e|e\rangle \rightarrow$$
$$\rightarrow |\psi\rangle = \tilde{c}_1|g_1\rangle + \tilde{c}_2|g_2\rangle + c_e|e\rangle \quad (11)$$

Where $\tilde{c}_i = c_i e^{-j\omega_i t}$ .

The extra factors add $\hbar\omega_i$ to the states $g_i$ , so the free atomic Hamiltonian changes to:

$$\tilde{H}_A = \frac{\vec{p}^2}{2m} - \hbar(\omega_{01} - \omega_1)|g_1\rangle\langle g_1| - \hbar(\omega_{02} - \omega_2)|g_2\rangle\langle g_2| =$$
$$= \frac{\vec{p}^2}{2m} + \hbar\Delta_1|g_1\rangle\langle g_1| + \hbar\Delta_2|g_2\rangle\langle g_2| \quad (12)$$

Note that $\Delta_i < 0$ , hence the sign in the above expression.

Next, update the field components as:

$$\tilde{E}_i^{(+)} = E_i^{(+)} e^{j\omega_i t}$$
$$\tilde{E}_i^{(-)} = E_i^{(-)} e^{-j\omega_i t} \quad (13)$$

Resulting atom-field Hamiltonian is then given by:

$$\tilde{H}_{AF} = \frac{\hbar}{2}\left[\Omega_1(\vec{r},\vec{k}_1)\sigma_1 + \Omega_1^*(\vec{r},\vec{k}_1)\sigma_1^\dagger\right] + \frac{\hbar}{2}\left[\Omega_2(\vec{k}_2)\sigma_2 + \Omega_2^*(\vec{k}_2)\sigma_2^\dagger\right] \quad (14)$$

Before the next step we neglect spontaneous emission i.e. assume $\Delta_i \gg \Gamma$, where $\Gamma$ is spontaneous decay rate of the excited state. I.e. our time scales are (much) slower than $1/\Gamma$ .

## S1.3: Deriving the Schrodinger equation and extracting 2-level dynamics

We wish to solve Schrodinger's equation for

$$i\hbar\partial_t|\psi\rangle = (\tilde{H}_A + \tilde{H}_{AF})|\psi\rangle \quad (15)$$

Where $|\psi\rangle$ is a super-position of tensor products of internal and external states in the field's rotating frames:

$$|\psi\rangle = |\psi_{g1}\rangle|g_1\rangle + |\psi_{g2}\rangle|g_2\rangle + |\psi_e\rangle|e\rangle \quad (16)$$

Substitute the above general state into (15):

$$i\hbar\partial_t\left(|\psi_{g1}\rangle|g_1\rangle + |\psi_{g2}\rangle|g_2\rangle + |\psi_e\rangle|e\rangle\right) = (\tilde{H}_A + \tilde{H}_{AF})\left(|\psi_{g1}\rangle|g_1\rangle + |\psi_{g2}\rangle|g_2\rangle + |\psi_e\rangle|e\rangle\right) \Rightarrow$$
$$\Rightarrow i\hbar\partial_t|\psi_{g1}\rangle|g_1\rangle + i\hbar\partial_t|\psi_{g2}\rangle|g_2\rangle + i\hbar\partial_t|\psi_e\rangle|e\rangle =$$
$$= \left(\frac{\vec{p}^2}{2m} + \hbar\Delta_1|g_1\rangle\langle g_1| + \hbar\Delta_2|g_2\rangle\langle g_2| + \frac{\hbar}{2}\left[\Omega_1(\vec{r})|g_1\rangle\langle e| + \Omega_1^*(\vec{r})|e\rangle\langle g_1|\right] + \frac{\hbar}{2}\left[\Omega_2(\vec{r})|g_2\rangle\langle e| + \Omega_2^*(\vec{r})|e\rangle\langle g_2|\right]\right)$$
$$\left(|\psi_{g1}\rangle|g_1\rangle + |\psi_{g2}\rangle|g_2\rangle + |\psi_e\rangle|e\rangle\right) \Rightarrow$$

$$\Rightarrow \begin{cases} i\hbar\partial_t|\psi_{g1}\rangle|g_1\rangle = \left(\frac{\vec{p}^2}{2m} + \hbar\Delta_1\right)|\psi_{g1}\rangle|g_1\rangle + \frac{\hbar\Omega_1(\vec{r})}{2}|\psi_e\rangle|g_1\rangle \\ i\hbar\partial_t|\psi_{g2}\rangle|g_2\rangle = \left(\frac{\vec{p}^2}{2m} + \hbar\Delta_2\right)|\psi_{g2}\rangle|g_2\rangle + \frac{\hbar\Omega_2(\vec{r})}{2}|\psi_e\rangle|g_2\rangle \\ i\hbar\partial_t|\psi_e\rangle|e\rangle = \frac{\vec{p}^2}{2m}|\psi_e\rangle|e\rangle + \frac{\hbar\Omega_1^*(\vec{r})}{2}|\psi_{g1}\rangle|e\rangle + \frac{\hbar\Omega_2^*(\vec{r})}{2}|\psi_{g2}\rangle|e\rangle \end{cases} \quad (17)$$

We arrive at equation of motion for the external states:

$$i\hbar\partial_t\left|\psi_{g1}\right\rangle=\left(\frac{\vec{p}^2}{2m}+\hbar\Delta_1\right)\left|\psi_{g1}\right\rangle+\frac{\hbar\Omega_1\left(\vec{r},\vec{k}_1\right)}{2}\left|\psi_e\right\rangle$$

$$i\hbar\partial_t\left|\psi_{g2}\right\rangle=\left(\frac{\vec{p}^2}{2m}+\hbar\Delta_2\right)\left|\psi_{g2}\right\rangle+\frac{\hbar\Omega_2\left(\vec{k}_2\right)}{2}\left|\psi_e\right\rangle \qquad (18)$$

$$i\hbar\partial_t\left|\psi_e\right\rangle=\frac{\vec{p}^2}{2m}\left|\psi_e\right\rangle\left|e\right\rangle+\frac{\hbar\Omega_1^*\left(\vec{r},\vec{k}_1\right)}{2}\left|\psi_{g1}\right\rangle+\frac{\hbar\Omega_2^*\left(\vec{k}_2\right)}{2}\left|\psi_{g2}\right\rangle$$

Adding $-\hbar\Delta=-\frac{\hbar}{2}\left(\Delta_1+\Delta_2\right)$ to all the energies and get:

$$i\hbar\partial_t\left|\psi_{g1}\right\rangle=\left(\frac{\vec{p}^2}{2m}+\hbar\Delta_1\right)\left|\psi_{g1}\right\rangle+\frac{\hbar\Omega_1\left(\vec{r},\vec{k}_1\right)}{2}\left|\psi_e\right\rangle-\frac{\hbar}{2}\left(\Delta_1+\Delta_2\right)\left|\psi_{g1}\right\rangle$$

$$i\hbar\partial_t\left|\psi_{g2}\right\rangle=\left(\frac{\vec{p}^2}{2m}+\hbar\Delta_2\right)\left|\psi_{g2}\right\rangle+\frac{\hbar\Omega_2\left(\vec{k}_2\right)}{2}\left|\psi_e\right\rangle-\frac{\hbar}{2}\left(\Delta_1+\Delta_2\right)\left|\psi_{g2}\right\rangle \qquad \Rightarrow$$

$$i\hbar\partial_t\left|\psi_e\right\rangle=\frac{\vec{p}^2}{2m}\left|\psi_e\right\rangle\left|e\right\rangle+\frac{\hbar\Omega_1^*\left(\vec{r},\vec{k}_1\right)}{2}\left|\psi_{g1}\right\rangle+\frac{\hbar\Omega_2^*\left(\vec{k}_2\right)}{2}\left|\psi_{g2}\right\rangle-\frac{\hbar}{2}\left(\Delta_1+\Delta_2\right)\left|\psi_e\right\rangle \qquad (19)$$

$$i\hbar\partial_t\left|\psi_{g1}\right\rangle=\frac{\vec{p}^2}{2m}\left|\psi_{g1}\right\rangle+\frac{\hbar\Omega_1\left(\vec{r},\vec{k}_1\right)}{2}\left|\psi_e\right\rangle+\hbar\left(\Delta_1-\Delta\right)\left|\psi_{g1}\right\rangle$$

$$\Rightarrow \qquad i\hbar\partial_t\left|\psi_{g2}\right\rangle=\frac{\vec{p}^2}{2m}\left|\psi_{g2}\right\rangle+\frac{\hbar\Omega_2\left(\vec{k}_2\right)}{2}\left|\psi_e\right\rangle+\hbar\left(\Delta_2-\Delta\right)\left|\psi_{g2}\right\rangle$$

$$i\hbar\partial_t\left|\psi_e\right\rangle=\frac{\vec{p}^2}{2m}\left|\psi_e\right\rangle\left|e\right\rangle+\frac{\hbar\Omega_1^*\left(\vec{r},\vec{k}_1\right)}{2}\left|\psi_{g1}\right\rangle+\frac{\hbar\Omega_2^*\left(\vec{k}_2\right)}{2}\left|\psi_{g2}\right\rangle-\hbar\Delta\left|\psi_e\right\rangle$$

Applying adiabatic elimination along with assumption of large enough detuning we get for the third equation in (19):

$$0\approx i\hbar\partial_t\left|\psi_e\right\rangle=\frac{\vec{p}^2}{2m}\left|\psi_e\right\rangle\left|e\right\rangle+\frac{\hbar\Omega_1^*\left(\vec{r},\vec{k}_1\right)}{2}\left|\psi_{g1}\right\rangle+\frac{\hbar\Omega_2^*\left(\vec{k}_2\right)}{2}\left|\psi_{g2}\right\rangle-\hbar\Delta\left|\psi_e\right\rangle\Rightarrow$$

$$\Rightarrow\left|\psi_e\right\rangle=\frac{\Omega_1^*\left(\vec{r},\vec{k}_1\right)}{2\Delta}\left|\psi_{g1}\right\rangle+\frac{\Omega_2^*\left(\vec{k}_2\right)}{2\Delta}\left|\psi_{g2}\right\rangle \qquad (20)$$

Substitute back into (19) for the equation of motion for the ground states and remove the $-\hbar\Delta = -\frac{\hbar}{2}\left(\Delta_1 + \Delta_2\right)$ from all energies:

$$\begin{aligned} i\hbar\partial_t\left|\psi_{g1}\right\rangle &= \frac{\vec{p}^2}{2m}\left|\psi_{g1}\right\rangle + \frac{\hbar\Omega_1(\vec{r})}{2}\left(\frac{\Omega_1^*(\vec{r})}{2\Delta}\left|\psi_{g1}\right\rangle + \frac{\Omega_2^*(\vec{r})}{2\Delta}\left|\psi_{g2}\right\rangle\right) + \hbar\left(\Delta_1 - \Delta\right)\left|\psi_{g1}\right\rangle \\ i\hbar\partial_t\left|\psi_{g2}\right\rangle &= \frac{\vec{p}^2}{2m}\left|\psi_{g2}\right\rangle + \frac{\hbar\Omega_2(\vec{r})}{2}\left(\frac{\Omega_1^*(\vec{r})}{2\Delta}\left|\psi_{g1}\right\rangle + \frac{\Omega_2^*(\vec{r})}{2\Delta}\left|\psi_{g2}\right\rangle\right) + \hbar\left(\Delta_2 - \Delta\right)\left|\psi_{g2}\right\rangle \end{aligned} \Rightarrow$$

$$\Rightarrow \begin{aligned} i\hbar\partial_t\left|\psi_{g1}\right\rangle &= \left[\frac{\vec{p}^2}{2m} + \hbar\Delta_1 + \frac{\hbar\left|\Omega_1(\vec{r})\right|^2}{4\Delta}\right]\left|\psi_{g1}\right\rangle + \frac{\hbar\Omega_1(\vec{r})\Omega_2^*(\vec{r})}{4\Delta}\left|\psi_{g2}\right\rangle \\ i\hbar\partial_t\left|\psi_{g2}\right\rangle &= \left[\frac{\vec{p}^2}{2m} + \hbar\Delta_2 + \frac{\hbar\left|\Omega_2(\vec{r})\right|^2}{4\Delta}\right]\left|\psi_{g2}\right\rangle + \frac{\hbar\Omega_1^*(\vec{r})\Omega_2(\vec{r})}{4\Delta}\left|\psi_{g1}\right\rangle \end{aligned} \quad (21)$$

## S1.4: Defining the Raman Rabi frequency

Using (21), we can define the Raman Rabi frequency:

$$\Omega_R(\vec{r}) = \frac{\Omega_1(\vec{r})\Omega_2^*(\vec{r})}{2\Delta} \quad (22)$$

And AC Stark shifts:

$$\omega_{AC,i} = \frac{\Omega_i^2}{4\Delta} \Rightarrow$$

$$\Rightarrow \begin{aligned} \frac{\Omega_1^2}{4\Delta} &= \frac{\left|\left\langle g_1\right|\vec{d}\left|e\right\rangle \cdot \vec{\tilde{E}}_1(\vec{r})\right|^2}{4\Delta\hbar^2} \\ \frac{\Omega_2^2}{4\Delta} &= \frac{\left|\left\langle g_2\right|\vec{d}\left|e\right\rangle \cdot \vec{\tilde{E}}_2(\vec{r})\right|^2}{4\Delta\hbar^2} \end{aligned} \quad (23)$$

With help of (22) and (23) we rewrite (21):

$$\begin{aligned} i\hbar\partial_t\left|\psi_{g1}\right\rangle &= \left[\frac{\vec{p}^2}{2m} + \hbar\Delta_1 + \hbar\omega_{AC,1}(\vec{r})\right]\left|\psi_{g1}\right\rangle + \frac{\hbar\Omega_R(\vec{r})}{2}\left|\psi_{g2}\right\rangle \\ i\hbar\partial_t\left|\psi_{g2}\right\rangle &= \left[\frac{\vec{p}^2}{2m} + \hbar\Delta_2 + \hbar\omega_{AC,2}(\vec{r})\right]\left|\psi_{g2}\right\rangle + \frac{\hbar\Omega_R^*(\vec{r})}{2}\left|\psi_{g1}\right\rangle \end{aligned} \quad (24)$$

The Raman Hamiltonian for effective 2-level system becomes:

$$H_R = \frac{\vec{p}^2}{2m} + \hbar\left(\Delta_1 + \hbar\omega_{AC,1}\left(\vec{r}\right)\right)\left|g_1\right\rangle\left\langle g_1\right| + \hbar\left(\Delta_2 + \hbar\omega_{AC,2}\left(\vec{r}\right)\right)\left|g_2\right\rangle\left\langle g_2\right| +$$

$$+\frac{\hbar}{2}\left(\Omega_R^*\left(\vec{r}\right)\left|g_1\right\rangle\left\langle g_2\right| + \Omega_R\left(\vec{r}\right)\left|g_2\right\rangle\left\langle g_1\right|\right) = \tag{25}$$

$$= \frac{\vec{p}^2}{2m} + \hbar\left(\Delta_1 + \hbar\omega_{AC,1}\left(\vec{r}\right)\right)\left|g_1\right\rangle\left\langle g_1\right| + \hbar\left(\Delta_2 + \hbar\omega_{AC,2}\left(\vec{r}\right)\right)\left|g_2\right\rangle\left\langle g_2\right| + \frac{\hbar}{2}\left(\Omega_R^*\left(\vec{r}\right)\sigma_R + \Omega_R\left(\vec{r}\right)\sigma_R^\dagger\right)$$

## S2: Dipole matrix element calculation

We now go back to (8) for a detailed calculation of the matrix element:

$$\vec{r}\cdot\hat{u}_q = \sqrt{\frac{4\pi}{3}} r Y_{1,q}\left(\theta,\phi\right) \Rightarrow$$

$$\Rightarrow \left\langle g_\alpha\right|\vec{d}\cdot\hat{u}_q\left|e\right\rangle = -q_e \iiint r^2 \sin\theta dr d\theta d\phi \left[\psi_{g_\alpha}^*\left(r,\theta,\phi\right)\sqrt{\frac{4\pi}{3}} r Y_{1,q}\left(\theta,\phi\right)\psi_e\left(r,\theta,\phi\right)\right]$$

For the simple system without hyper-fine or fine splitting, we can split the above integral into radial part (or in more general way reduced matrix element) and angular part. The radial part is of the form $\left\langle \alpha' L'\right\|r\left\|\alpha L\right\rangle$ where L is general orbital angular momentum, note that this part's quantum number dependence stays the same both for fine structure and hyper-fine structure, since light couples only to the orbital angular momentum and doesn't couple to the spin. For the angular part we write:

$$\begin{aligned}&\left\langle F'J'M_F'\right|\vec{d}\cdot\hat{u}_q\left|FJM_F\right\rangle = \\ &= -q_e\left(-1\right)^{1+L'+S+J+J'+I-M_F'}\sqrt{\left(2J+1\right)\left(2J'+1\right)\left(2F+1\right)\left(2F'+1\right)}\times \\ &\times\begin{Bmatrix} L' & J' & S \\ J & L & 1\end{Bmatrix}\begin{Bmatrix} J' & F' & I \\ F & J & 1\end{Bmatrix}\begin{pmatrix} F & 1 & F' \\ M_F & q & M_F'\end{pmatrix}\end{aligned} \tag{26}$$

Where $I$ is the nuclear spin $F = L + S + I$ and $J = L + S$ . Elements in curly brackets are Wigner 6j symbol and in regular brackets are Wigner 3j symbol.

Overall matrix element is then of the form:

$$\begin{aligned}&\left\langle g_\alpha\right|\vec{d}\cdot\hat{u}_q\left|e\right\rangle = \\ &= -q_e\left(-1\right)^{1+L'+S+J+J'+I-M_F'}\sqrt{\left(2J+1\right)\left(2J'+1\right)\left(2F+1\right)\left(2F'+1\right)}\times \\ &\times\begin{Bmatrix} L' & J' & S \\ J & L & 1\end{Bmatrix}\begin{Bmatrix} J' & F' & I \\ F & J & 1\end{Bmatrix}\times \\ &\times\begin{pmatrix} F & 1 & F' \\ M_F & q & M_F'\end{pmatrix}\left\langle n_s^* L'\right\|r\left\|n_p^* L\right\rangle\end{aligned} \tag{27}$$

For $^{40}$K we consider $4s$ to $4p$ transition between ground states and an exited state. For the radial part $\langle \alpha' L' \| r \| \alpha L \rangle$ can be written as $\langle n_s^* s \| r \| n_p^* p \rangle$ where $n_s^* = 1.77,\ n_p^* = 2.235$. Since alkali-metal atoms like Potassium have only one active electron we can now treat this matrix element as hydrogen-like element with the above quantum numbers.

## S2.1: Selection rules

Recall the generalized Raman frequency given by (22):

$$\Omega_R(\vec{r}) = \frac{\Omega_1(\vec{r})\Omega_2^*(\vec{r})}{2\Delta} = \frac{1}{2\Delta\hbar^2}\left[\langle g_1|\vec{d}|e\rangle \cdot \tilde{\vec{E}}_1^*(\vec{r})\right]\left[\langle g_2|\vec{d}|e\rangle \cdot \tilde{\vec{E}}_2(\vec{r})\right] \quad (29)$$

We wish to rewrite it by using (4.5):

$$\begin{aligned}
\Omega_R(\vec{r}) &= \frac{1}{2\Delta\hbar^2}\left[\langle g_1|\vec{d}|e\rangle \cdot \tilde{\vec{E}}_1^*(\vec{r})\right]\left[\langle g_2|\vec{d}|e\rangle \cdot \tilde{\vec{E}}_2(\vec{r})\right] \\
&= \frac{1}{4\Delta\hbar^2}\left\{\langle g_1|\vec{d}\cdot\hat{u}_{+1}|e\rangle\left[\tilde{E}_{1,x}^*(\vec{r}) - i\tilde{E}_{1,y}^*(\vec{r})\right] + \frac{1}{\sqrt{2}}\langle g_1|\vec{d}\cdot\hat{u}_{-1}|e\rangle\left[\tilde{E}_{1,x}^*(\vec{r}) + i\tilde{E}_{1,y}^*(\vec{r})\right] + \langle g_1|\vec{d}\cdot\hat{u}_0|e\rangle\tilde{E}_{1,z}^*(\vec{r})\right\}\times \quad (30) \\
&\times\left\{\langle g_2|\vec{d}\cdot\hat{u}_{+1}|e\rangle\left[\tilde{E}_{2,x}(\vec{r}) - i\tilde{E}_{2,y}(\vec{r})\right] + \frac{1}{\sqrt{2}}\langle g_2|\vec{d}\cdot\hat{u}_{-1}|e\rangle\left[\tilde{E}_{2,x}(\vec{r}) + i\tilde{E}_{2,y}(\vec{r})\right] + \langle g_2|\vec{d}\cdot\hat{u}_0|e\rangle\tilde{E}_{2,z}(\vec{r})\right\}
\end{aligned}$$

Looking at the single expression of the form $\langle g_1|\vec{d}\cdot\hat{u}_{q_1}|e\rangle\langle g_2|\vec{d}\cdot\hat{u}_{q_2}|e\rangle$ where $q_i$ is the polarization component of the driving field $\vec{E}_i$ and by using (27):

$$\begin{aligned}
&\langle g_1|\vec{d}\cdot\hat{u}_{q_1}|e\rangle\langle g_2|\vec{d}\cdot\hat{u}_{q_2}|e\rangle = \\
&= q_e^2(-1)^{1+L_1+S_e+J_e+J_1+I-M_{F,1}}\sqrt{(2J_e+1)(2J_1+1)(2F_e+1)(2F_1+1)}\begin{Bmatrix} L_1 & J_1 & S_e \\ J_e & L_e & 1 \end{Bmatrix}\begin{Bmatrix} J_1 & F_1 & I_e \\ F_e & J_e & 1 \end{Bmatrix}\times \\
&\times\begin{pmatrix} F_e & 1 & F_1 \\ M_{F,e} & q_1 & M_{F,1} \end{pmatrix}\langle n_s^* L_1\|r\|n_p^* L_e\rangle\times \quad (31) \\
&\times(-1)^{1+L_2+S_e+J_e+J_2+I-M_{F,2}}\sqrt{(2J_e+1)(2J_2+1)(2F_e+1)(2F_2+1)}\begin{Bmatrix} L_2 & J_2 & S_e \\ J_e & L_e & 1 \end{Bmatrix}\begin{Bmatrix} J_2 & F_2 & I_e \\ F_e & J_e & 1 \end{Bmatrix}\times \\
&\times\begin{pmatrix} F_e & 1 & F_2 \\ M_{F,e} & q_2 & M_{F,2} \end{pmatrix}\langle n_s^* L_2\|r\|n_p^* L_e\rangle
\end{aligned}$$

where the subscript of quantum number $N$ corresponds to quantum number belonging to $|g_2\rangle, |g_1\rangle$ and $|e\rangle$, respectively.

By assuming that $|g_1\rangle$ and $|g_2\rangle$ states are Zeeman states, they differ only by their magnetic number $M_F$, in which case (31) becomes:

$$\langle g_1|\vec{d}\cdot\hat{u}_{q_1}|e\rangle\langle g_2|\vec{d}\cdot\hat{u}_{q_2}|e\rangle =$$
$$= q_e^2\left|\langle n_s^*L\|r\|n_p^*L_e\rangle\right|^2(-1)^{2+2L+2S_e+2J_e+2J+2I-M_{F,1}-M_{F,2}}\left[(2J_e+1)(2J+1)(2F_e+1)(2F+1)\right]\times$$
$$\times\begin{Bmatrix} L & J & S_e \\ J_e & L_e & 1 \end{Bmatrix}^2\begin{Bmatrix} J & F & I_e \\ F_e & J_e & 1 \end{Bmatrix}^2\times \quad (32)$$
$$\times\begin{pmatrix} F_e & 1 & F \\ M_{F,e} & q_1 & M_{F,1} \end{pmatrix}\begin{pmatrix} F_e & 1 & F \\ M_{F,e} & q_2 & M_{F,2} \end{pmatrix}$$

Note that Wigner 3j symbol of the form $\begin{pmatrix} F_e & 1 & F \\ M_{F,e} & q_i & M_{F,i} \end{pmatrix}$ needs to satisfy the following:

$$M_{F,e}+q_i+M_{F,i}=0 \text{ and } |F_e-1|\le F\le F_e+1 \quad (33)$$

By substituting the first constraint into the last term in (32) we get:

$$\begin{cases} M_{F,e}+q_1+M_{F,1}=0 \\ M_{F,e}+q_2+M_{F,2}=0 \end{cases}\Rightarrow q_1+M_{F,1}=q_2+M_{F,2} \quad (34)$$

By looking at our assumptions on quantum numbers relations we can further write:

$$\begin{cases} M_{F,e}+q_1+M_{F,1}=0 \\ M_{F,e}+q_2+M_{F,2}=0 \end{cases}\Rightarrow q_1+M_{F,1}=q_2+M_{F,2}\Rightarrow q_1+M_{F,2}-1=q_2+M_{F,2}\Rightarrow q_2=q_1-1 \quad (35)$$

Rewriting (32) with help of the (35, yields us with:

$$\langle g_1|\vec{d}\cdot\hat{u}_{q_1}|e\rangle\langle g_2|\vec{d}\cdot\hat{u}_{q_2}|e\rangle =$$
$$= q_e^2\left|\langle n_s^*L\|r\|n_p^*L_e\rangle\right|^2(-1)^{1+2\left[L+S+J_e+J+I-M_{F,1}\right]}\left[(2J_e+1)(2J+1)(2F_e+1)(2F+1)\right]\times$$
$$\times\begin{Bmatrix} L & J & S \\ J_e & L_e & 1 \end{Bmatrix}^2\begin{Bmatrix} J & F & I_e \\ F_e & J_e & 1 \end{Bmatrix}^2\times \quad (36)$$
$$\times\begin{pmatrix} F_e & 1 & F \\ M_{F,e} & q_1 & M_{F,1} \end{pmatrix}\begin{pmatrix} F_e & 1 & F \\ M_{F,e} & q_1-1 & M_{F,1}+1 \end{pmatrix}$$

It is possible to build "coupling ladder" which tells us which polarization from field $\vec{E}_1$ couples to which polarization from field $\vec{E}_2$ and vice versa. As long as our states $|g_2\rangle, |g_1\rangle$ and $|e\rangle$ are valid quantum states, this table will define selection rules in our system:

$$\boxed{\begin{array}{ccc} q_1 & & q_2 \\ \varnothing & \leftrightarrow & +1 \\ +1 & \leftrightarrow & 0 \\ 0 & \leftrightarrow & -1 \\ -1 & \leftrightarrow & \varnothing \end{array}} \quad (37)$$

where $\varnothing$ symbol indicates "ladder cut".

Rewriting (29) with (37) and (36), the only terms of the form in (37) will contribute non-zero matrix elements (note that matrix elements themselves are real numbers):

$$\begin{aligned}
\Omega_R(\vec{r}) &= \frac{1}{2\Delta\hbar^2}\Big[\langle g_1|\vec{d}|e\rangle\cdot\vec{\tilde{E}}_1^*(\vec{r})\Big]\Big[\langle g_2|\vec{d}|e\rangle\cdot\vec{\tilde{E}}_2(\vec{r})\Big] \\
&= \frac{1}{4\Delta\hbar^2}\left\{\begin{array}{l}\langle g_1|\vec{d}\cdot\hat{u}_{+1}|e\rangle\Big[\tilde{E}_{1,x}^*(\vec{r})+i\tilde{E}_{1,y}^*(\vec{r})\Big]+ \\ +\frac{1}{\sqrt{2}}\langle g_1|\vec{d}\cdot\hat{u}_{-1}|e\rangle\Big[\tilde{E}_{1,x}^*(\vec{r})-i\tilde{E}_{1,y}^*(\vec{r})\Big]+\langle g_1|\vec{d}\cdot\hat{u}_0|e\rangle\tilde{E}_{1,z}^*(\vec{r})\end{array}\right\}\times \\
&\times\left\{\begin{array}{l}\langle g_2|\vec{d}\cdot\hat{u}_{+1}|e\rangle\Big[\tilde{E}_{2,x}(\vec{r})-i\tilde{E}_{2,y}(\vec{r})\Big]+ \\ +\frac{1}{\sqrt{2}}\langle g_2|\vec{d}\cdot\hat{u}_{-1}|e\rangle\Big[\tilde{E}_{2,x}(\vec{r})+i\tilde{E}_{2,y}(\vec{r})\Big]+\langle g_2|\vec{d}\cdot\hat{u}_0|e\rangle\tilde{E}_{2,z}(\vec{r})\end{array}\right\}= \\
&= \frac{1}{4\sqrt{2}\Delta\hbar^2}\Big\{\langle g_1|\vec{d}\cdot\hat{u}_{+1}|e\rangle\langle g_2|\vec{d}\cdot\hat{u}_0|e\rangle\Big[\tilde{E}_{1,x}(\vec{r})-i\tilde{E}_{1,y}(\vec{r})\Big]^*\Big[\tilde{E}_{2,z}(\vec{r})\Big]\Big\}+ \\
&+\frac{1}{4\sqrt{2}\Delta\hbar^2}\Big\{\langle g_1|\vec{d}\cdot\hat{u}_0|e\rangle\langle g_2|\vec{d}\cdot\hat{u}_{-1}|e\rangle\Big[\tilde{E}_{1,z}(\vec{r})\Big]^*\Big[\tilde{E}_{2,x}(\vec{r})+i\tilde{E}_{2,y}(\vec{r})\Big]\Big\}
\end{aligned} \quad (38)$$

Rewriting the (38) we arrive at the expression given in main text:

$$\begin{aligned}
&4\sqrt{2}\Delta\hbar^2\Omega_R\left(\vec{r},\vec{k}_1,\vec{k}_2\right)= \\
&= M_{+1,0}\Big[\tilde{E}_{1,x}\left(\vec{r},\vec{k}_1\right)-i\tilde{E}_{1,y}\left(\vec{r},\vec{k}_1\right)\Big]\tilde{E}_{2,z}^*\left(\vec{r},\vec{k}_2\right)+M_{0,-1}\Big[\tilde{E}_{2,x}^*\left(\vec{r},\vec{k}_2\right)-i\tilde{E}_{2,y}^*\left(\vec{r},\vec{k}_2\right)\Big]\tilde{E}_{1,z}\left(\vec{r},\vec{k}_1\right)
\end{aligned} \quad (39)$$

where $M_{q_1,q_2} = \langle g_1|\vec{d}\cdot\hat{u}_{q_1}|e\rangle\langle g_2|\vec{d}\cdot\hat{u}_{q_2}|e\rangle$ .

## S3: Topological charge calculation

From main text we use the following expression for the Pontryagin number:

$$S = \frac{1}{4\pi}\iint_A \vec{m}\cdot\left(\frac{\partial \vec{m}}{\partial x}\times\frac{\partial \vec{m}}{\partial y}\right)dA \quad (40)$$

In order to calculate how Pontryagin number changes as we increase the domain of integration from the center of the unit cell to its boundary we need to define a sequence of domains $\{A_i\}_{i=0}^{N}$ so that $\bigcup_{i=0}^{N} A_i$ is the unit cell. We note that the boundary of the unit cell has hexagonal shape and inner part of the unit cell has a round shape, therefore we define the following:

$$\begin{aligned}
&R_i = 0.6055\lambda_0 \frac{i}{N} \\
&B:\left\{(x,y)\middle\|x\right| < 0.5245\lambda_0,\ \text{-}0.5767x + 0.6055\lambda_0 < |y| < 0.5767x + 0.6055\lambda_0\right\} \quad (41) \\
&A_i:\left\{(x,y)\middle| x^2 + y^2 < R_i\right\}\cap B
\end{aligned}$$

Where $(x,y)$ normalized with respect to $\lambda_0$. Domain $B$ corresponds to the hexagonal boundary of the unit cell and is calculated by applying periodic condition of the lattice.

Using (41) we calculate $N+1$ values of (40) where for main text we chose $N+1=1000$.

## S4: A note on wavelengths

Spinor states $|g_1\rangle$ and $|g_2\rangle$ are non-degenerate Zeeman splitted states, hence the frequency between them is set by a magnetic field. Typical value for such splitting is around $50\ [MHz]$, around the Feshbach resonance at $202.14\ [Gauss]$. Therefore the wavelengths of the Raman fields can be chosen to be very close to each other so that the lattice structure of the spin textures will not be distorted for up to $\sim 1000$ lattice sites.
